# Supplementary material for: Looking at words and points with attention: a benchmark for text-to-shape coherence
Source: arXiv:2309.07917 source file (2023-09-14)
Supplement: Supplementary file 1 [file ai3dcc_supplementary.pdf]

# Supplementary for Looking at words and points with attention: a benchmark for text-to-shape coherence


Andrea Amaduzzi   Giuseppe Lisanti   Samuele Salti   Luigi Di Stefano

CVLAB, Department of Computer Science and Engineering (DISI)
University of Bologna, Italy

{andrea.amaduzzi4, giuseppe.lisanti, samuele.salti, luigi.distefano}@unibo.it


## A. AutoEncoder Architecture

As mentioned in Section 4 of the main paper, in order to build the `reference-distractor-text` triplets for the user study, we relied on the Euclidean distance in the latent space of a PointNet++ autoencoder [6], trained on the task of 3D reconstruction. Furthermore, the point cloud features used in the cross-attention mechanism of our CrossCoherence metric have been taken from this autoencoder, as highlighted in Figure 1.

This architecture is composed of a PointNet++ [6] encoder made out of three set abstraction layers with multi-scale grouping (MSG) and a transformation network T-Net [5], and a simple convolutional decoder, made of three stacked $1 \times 1$ convolutions with ReLUs in between. Differently from a standard PointNet++, the input of this network is an RGB point cloud featuring spatial coordinates *(x, y, z)* and colors *(R, G, B)*, which are used as input features for every point.

The model has been trained on the task of shape reconstruction on the chair and table categories of the ShapeNet dataset [1]. In order to build the *easy* and *hard* shape distractors, we extracted the shape embeddings from the third set-abstraction layer, which is a global feature vector of dimension 1024. For the CrossCoherence metric, the shape embedding has been taken from the features output of the second set-abstraction layer, which has dimension $128 \times 640$.

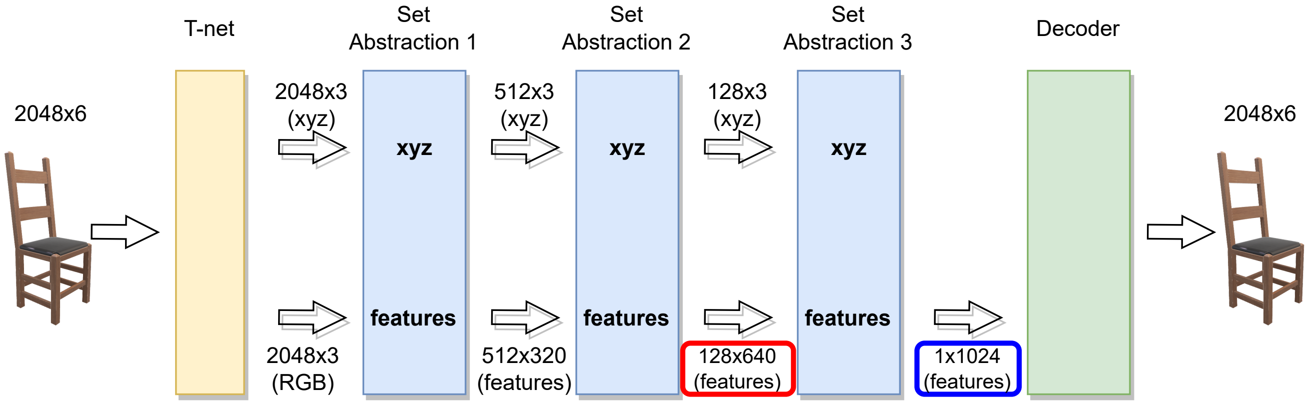


Figure 1. Architecture of the PointNet++ autoencoder. In **red** the features used by CrossCoherence, and in **blue** the embeddings that have been used to compute the *easy* and *hard* distractors for each reference shape.

## B. Examples of GPT2Shape text prompts

In this section, we provide additional examples of text prompts from Text2Shape and GPT2Shape. As discussed in the main paper, the text generation method put forth in this work enables to obtain more informative sentences from the shape descriptions available in Text2Shape, which oftentimes are equivocal and inconsistent. Figure 2 shows GPT2Shape text prompts with correct and comprehensive information, together with the corresponding original prompts from Text2Shape.

We can clearly notice the lack of details in the descriptions of Text2Shape, whereas the rephrased descriptions can capture all the relevant geometric and appearance details of the 3D shapes. Nonetheless, in a limited number of cases, the LLM (Large Language Model) used to generate the new descriptions, i.e. GPT-3, cannot produce text prompts of satisfactory quality. Figure 3 shows some cases where wrong information are still present in the text prompts of GPT2Shape. This occurs mainly due to inconsistencies present in the original dataset which are hard to remove, particularly if they are repeated throughout multiple sentences associated with the same shape, e.g. the color of the table in the middle (*black* or *navy*) and the inconsistency on the number of legs in the last example. Other minor errors are due to subtle details of the description, like the shape of the chair wrongly described as *rectangular* in the first example.

## C. *easy-hard* shape distractors

For every reference shape of GPT2Shape, we have defined two *hard* distractors and one *easy* distractor, on the basis of the Euclidean distance in the latent space of a PointNet++ [6]. In particular, the hard distractors were chosen to be the 2 shapes closest to the reference in terms of both geometry and colour, the easy distractor was a randomly sampled shape having a distance from the reference larger than the median distance across the whole set of shapes of the same class. In Figure 4, we provide some examples of these triplets of shapes. We can notice how the distance in the embedding space of our PointNet++ encoder effectively captures similarity of geometric features and colors. These distractors have been exploited to compose the triplets for the user study and the training process of the CrossCoherence metric, as described in Section 4 and in Section 6.2 of the main manuscript, respectively.

## D. Examples from the User Study

As explained in the main paper in Section 4, the user study was conducted with two goals. Firstly, to evaluate the quality of the GPT2Shape dataset; secondly, to build the human-validated shape-text (HST) dataset containing informative descriptions filtered out from Text2Shape and GPT2Shape test sets. Figure 5 shows some triplets *shape-text-shape* for which the users expressed an unambiguous consensus on one shape above the other. For this reason, such samples belong to the HST dataset. On the contrary, Figure 6 provides examples of triplets that received ambiguous responses from the users, i.e. different preferences over the most coherent shape (last row), or cases in which the users selected "*I cannot decide between the two objects*" (other rows).

## E. Additional Experimental Results

In this section, we provide additional results, both qualitative and quantitative, to validate the proposed metric, i.e., CrossCoherence.

### E.1. Sensitivity of CLIP-based metrics to different 3D representations

We have carried out a sensitivity study on the 3D representation adopted to compute CLIP-Similarity and CLIP R-precision, by comparing the results achieved on HST with renderings obtained from point clouds and meshes. The results are reported in Tables 1 and 2.

Both these results and those reported in Tables 4 and 5 of the main paper highlight the strong dependence of CLIP-based metrics on the used 3D data representation. In particular, Tables 1 and 2 suggest that point clouds should be transformed into meshes to enable effective evaluation of text-to-shape coherence. Conversely, CrossCoherence is designed to work natively on point clouds and can judge effectively upon this kind of data without requiring conversion into meshes. This behavior of CLIP-based metrics can make them less generalizable across different types of 3D data and potentially biased towards certain types of representations. This can lead to inaccurate similarity scores and limit the usefulness of such metrics in applications that require robust similarity measures.

| **Method** | **Data representation** | **Accuracy** on chairs (↑) | **Accuracy** on full HST (↑) |
|---|---|---|---|
| CLIP-Similarity | Mesh | **77.79**% | **77.06**% |
| CLIP-Similarity | Point cloud | 72.26% | 70.78% |

Table 1. Sensitivity study of CLIP-similarity to different 3D representations. The second column specifies the 3D representations used for the evaluation. The third column reports accuracy only on chairs, while the fourth column on both chairs and tables.

| Test set | Data representation | CLIP R-precision |
|---|---|---|
| HST chairs | Mesh | **9.38**% |
| HST chairs | Point cloud | 8.95% |
| full HST | Mesh | **9.87**% |
| full HST | Point cloud | 7.83% |

Table 2. Sensitivity study of CLIP R-precision to different 3D representations. The second column specifies the 3D representations used for the evaluation. The third column reports the results of CLIP R-precision.

### E.2. Sensitivity of CLIP-based metrics to CLIP base model and number of renderings.

Given the same 3D representation, the performance of CLIP-based metrics as text-shape coherence metrics is strongly influenced by two factors: first, the CLIP base model used to compute the image and text embeddings; second, the number of rendered views used to compute the metric. Table 3 summarizes the results of CLIP-Similarity obtained using two different CLIP models and considering 1 or 10 or 20 rendered views. We report the two CLIP models that provided the best performance, with *ViT-L 14* performing slightly better than *ViT-B 32*. The rendered views are obtained from the mesh of every 3D shape. The gap in performance between the best and worst configuration is larger than 6% for CLIP-Similarity..

| **CLIP base model** | **Number of rendered views** | **Accuracy** on chairs (↑) | **Accuracy** on full HST (↑) |
|---|---|---|---|
| ViT-B 32 | 1 | 73.46% | 70.51% |
| ViT-B 32 | 10 | 76.49% | 75.43% |
| ViT-B 32 | 20 | 77.14% | 75.89% |
| ViT-L 14 | 1 | 72.91% | 70.32% |
| ViT-L 14 | 10 | 77.03% | 76.73% |
| ViT-L 14 | 20 | **77.79**% | **77.06**% |

Table 3. Performance of CLIP-Similarity on HST dataset using different CLIP base models and a different number of rendered views.

Since both CLIP R-precision and CLIP Similarity rely on the same vision-language model (e.g., CLIP) the sensitivity issues we discussed earlier regarding CLIP Similarity also apply to CLIP R-precision. In other words, both metrics are sensitive to the data representation, the CLIP-base model and the number of rendered views.

### E.3. CrossCoherence with different attention schemes

In Table 4, we show the performance achieved by CrossCoherence using different attention schemes. In particular, we evaluated the following architectures:

1. *Without Attention*: in this architecture, the shape and text embeddings directly undergo an average pooling layer, before being concatenated. No attention layer is present.
2. *Bilateral Cross-Attention*: this is the original scheme for CrossCoherence, featuring two cross-attention layers where in the first one the queries of the attention maps are computed on the shape features, whereas the keys and values are obtained from the text embeddings, while in the second layer this computation is reversed. Finally, the resulting embeddings from both the layers are concatenated, after undergoing an average pooling layer.
3. *Self-Attention*: we replace the cross-attention layers with self-attention layers and perform pooling and concatenation of their results.
4. *Bilateral Self-Attention and Cross-Attention*: before performing cross-attention, we feed the queries of each layer into a self-attention layer (one for the shape features and one for the text features).
5. *Bilateral Cross-Attention and Feed-Forward*: after performing cross-attention, we process the queries of each layer with a feed-forward layer (one for the shape features and one for the text features).

The Table points out clearly that the proposed Bilateral Cross-Attention (first row) is more effective than all the other formulations considered in the experiments. This suggests that the Cross-Attention mechanism effectively captures meaningful

relationships between shape and text features, leading to improved performance. The models utilizing Self-Attention alone and the combination of Self-Attention and Cross-Attention achieved very similar results, just below the best architecture. Self-Attention allows the model to attend to different parts of the input sequence, but it seems to be less effective in capturing complex dependencies compared to Cross-Attention. However, when equipped with a cross-attention layer, the performance had very slight variations on both the subset and the full HST, suggesting that adding Cross-Attention in this configuration did not provide any substantial benefit. Interestingly, the combination of Cross-Attention and Feed-Forward yielded the second-highest accuracy on the chairs of HST, 80.28%, but obtained performance comparable to the other schemes on the full HST. Finally, the architecture without any attention layer achieved the lowest accuracy on both datasets.

These findings highlight the importance of carefully selecting attention mechanisms in the design of models, with Cross-Attention being a particularly valuable choice for this specific task.

| **Method** | **Architecture** | **Accuracy** on chairs ($\uparrow$) | **Accuracy** on full HST ($\uparrow$) |
|---|---|---|---|
| CrossCoherence | Without Attention | 75.95% | 74.54% |
| CrossCoherence | Cross-Attention | **81.04%** | **80.45%** |
| CrossCoherence | Self-Attention | 78.98% | 78.08% |
| CrossCoherence | Self-Attention and Cross-Attention | 78.76% | 78.40% |
| CrossCoherence | Cross-Attention and Feed-Forward | 80.28% | 77.66% |

Table 4. Comparison on the HST test set between CrossCoherence using different attention schemes. The second column specifies the kind of attention used in the model. The third column reports accuracy for models trained and tested only on chairs, while the fourth column shows the results for models trained and tested on both chairs and tables.

### E.4. Qualitative comparison on HST dataset

In Figure 7, we show additional qualitative results on the HST dataset comparing CLIP-Similarity and CrossCoherence. In particular, we show some text prompts for which CrossCoherence is able to predict the reference shape as the most coherent with the text, while CLIP-Similarity is fooled by the distractor. As it is possible to notice, CLIP-Similarity lacks the ability to capture crucial geometric details from the input text descriptions, which may be due to its dependence on global embeddings for both text and image. Furthermore, the model's predictions are heavily influenced by the colour and texture of the shape, potentially leading to incorrect results when the input shapes share the same color. CrossCoherence is instead capable of focusing on specific details present in the text prompt to correctly discriminate between pairs of shape with a similar macroscopic structure, in terms of both geometry and appearance, e.g., *"a square cup-like shape"* for the first example, *"rectangular table"* for the second and third examples, *"rounded back"* in the fourth example, *"two horizontal slots in the backrest"* for the fifth example, *"two connected legs"* in the last example.

Figure 8 shows examples where the prediction made by CrossCoherence is wrong, while CLIP-Similarity is able to predict the correct shape. In such cases, the shapes of reference and the distractor are very similar, and the difference in the description may be re-conducted to just a few words, in some cases even just one word. As already highlighted in Section 7.1 of the main paper, these failures may result from the inability of a single coherent word/shape component to direct the prediction toward a distinct object. Furthermore, the chosen 3D representation may be a reason for the failure cases. This may be because the number of points on the specific part of the shape that differs between the reference point cloud and the distractor is small. Consequently, the shape features extracted from this region may not be informative enough to guide the model toward the correct prediction. On these triplets, CLIP-Similarity is instead capable of predicting the reference shape. This may be due to the fact that, as mentioned before, this metric seems to give a lot of importance to the color of the 3D shape; therefore, when the reference and distractor shapes differ only for the color of some parts, CLIP embeddings are capable of capturing this information very well, leading to a more accurate prediction than CrossCoherence. Finally, Figure 9 shows some triplets where both CLIP-Similarity and CrossCoherence provide wrong predictions. In this case, colors are very similar when not identical between reference and distractor, making it harder also for CLIP-Similarity, and the correct decision hinges again on one text attribute, like *tall* in the third example or *low-sitting* in the last one, which both metrics struggle to recognize. The second example shows how both metrics do not seem to be able to correctly reason on numerical attributes, as they both prefer the table with three legs instead of four.

With regards to CLIP R-precision, Figure 10 shows some results where CrossCoherence predicts the groundtruth text for the given 3D shape, while CLIP R-precision provides a wrong prediction. These examples confirm the difficulty of CLIP-based metrics in understanding the relations existing between the words of the textual descriptions and the corresponding shape parts.

### E.5. Qualitative comparison on generated data

We finally provide some additional qualitative results of CrossCoherence, CLIP-Similarity and CLIP R-precision when used to evaluate text-to-shape coherence of text-conditioned 3D shape generation methods. Figure 11 illustrates the predictions of CrossCoherence and CLIP-Similarity on the point clouds generated by Point-E [4] (left column), Shap-E [2] (middle column) and Liu et al. [3] (right column). These qualitative examples confirm that, when the metrics disagree, coherence of the generated shape to the input text seems higher for Liu et al, an aspect that is correctly captured by CrossCoherence. Figure 12 shows examples of the text prompts predicted by CLIP R-precision and CrossCoherence for 3D shapes generated by Shap-E [2]. This figure illustrates that the predictions from CrossCoherence are more accurate and fine-grained that the ones from CLIP R-precision.

## References


[1] Angel X Chang, Thomas Funkhouser, Leonidas Guibas, Pat Hanrahan, Qixing Huang, Zimo Li, Silvio Savarese, Manolis Savva, Shuran Song, Hao Su, et al. Shapenet: An information-rich 3d model repository. *arXiv preprint arXiv:1512.03012*, 2015. 1

[2] Heewoo Jun and Alex Nichol. Shap-e: Generating conditional 3d implicit functions. *arXiv preprint arXiv:2305.02463*, 2023. 5

[3] Zhengzhe Liu, Yi Wang, Xiaojuan Qi, and Chi-Wing Fu. Towards implicit text-guided 3d shape generation. In *Proceedings of the IEEE/CVF Conference on Computer Vision and Pattern Recognition*, pages 17896–17906, 2022. 5

[4] Alex Nichol, Heewoo Jun, Prafulla Dhariwal, Pamela Mishkin, and Mark Chen. Point-e: A system for generating 3d point clouds from complex prompts. *arXiv preprint arXiv:2212.08751*, 2022. 5

[5] Charles R Qi, Hao Su, Kaichun Mo, and Leonidas J Guibas. Pointnet: Deep learning on point sets for 3d classification and segmentation. In *Proceedings of the IEEE conference on computer vision and pattern recognition*, pages 652–660, 2017. 1

[6] Charles Ruizhongtai Qi, Li Yi, Hao Su, and Leonidas J Guibas. Pointnet++: Deep hierarchical feature learning on point sets in a metric space. *Advances in neural information processing systems*, 30, 2017. 1, 2

**Text2Shape**

**GPT2Shape**

**Text2Shape:**

“brown, without handle model, wood material, home use.”

“brown color square shape wood material old model”

“a wooden chair with a square padded seat and four legs, the back has three horizontal wooden stripes”

“Wooden chair with 4 wooden legs and wooden back support.”

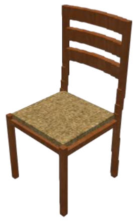

**GPT2Shape:**

“A square-shaped, brown wooden chair with four legs and a padded seat, featuring three horizontal wooden stripes on the back.”

“A brown, wood chair with a square seat and four legs, featuring a geometric design of three horizontal stripes on the back.”

“A home-use chair with a square seat and four legs, made of wood and featuring a brown color and three horizontal stripes on the back.”

“A wooden chair with a square seat, four legs, and a brown color, featuring a geometric design of three horizontal stripes on the back.”

**Text2Shape:**

“a blue and grey chair with a rectangular opening on its back.”

“Chair with blue legs and a grey back and seat. The back has a keyhole cut-out and the front and back legs are each connected.”

“A blue and maple finish designer chair for office or domestic use, very relaxing and inviting.”

“chair is made of fiber and cusion seat and back rest is fitted with cusion and it is in blue and grey color having four legs.”

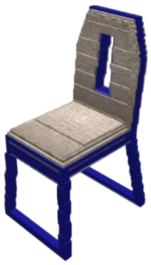

**GPT2Shape:**

“A blue and grey chair with a rectangular cut-out in the back, featuring four square legs and a cushion seat and backrest.”

“A designer chair with a blue and maple finish, featuring a grey cushion seat and backrest, and four square legs.”

“A relaxing and inviting chair with a grey cushion and blue borders, featuring a rectangular cut-out in the back and four square legs.”

“A comfortable chair with a grey cushion and blue borders, featuring a keyhole cut-out in the back and four conjoined legs.”

**Text2Shape:**

“A wooden table with thick rectangular top and has four slanted legs.”

“A rectangular shape wooden table with brown color.”

“The table is brown in color and has four inclined legs and the each pair is connected with a strip of metal rod.”

“wooden brown stripes and light brown colored table with supported legs joined with rods.”

“Long, rectangular wooden table with four slanted legs, like a foldout table. Legs are connected across the short axis with metal rods, and metal bolts are stuck in to the long sides of the front.”

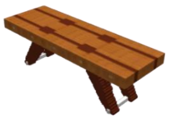

**GPT2Shape:**

“Rectangular wooden table with four slanted legs, brown in color with metal rods connecting the legs.”

“Long, brown rectangular table with four inclined legs connected by metal rods.”

“Thick, rectangular wooden table with four slanted legs, brown with light brown stripes.”

“Rectangular wooden table with four slanted legs, brown with metal rods connecting the legs.”

“Rectangular wooden table with four slanted legs, brown with light brown stripes and metal rods connecting the legs.”

Figure 2. Three examples of wrong Text2Shape prompts which are corrected in GTP2Shape. The green box contains the original Text2Shape descriptions for the 3D shape in the middle. The blue box shows the rephrased text prompts of GPT2Shape. In yellow, we highlight the ambiguous or wrong descriptions of Text2Shape.

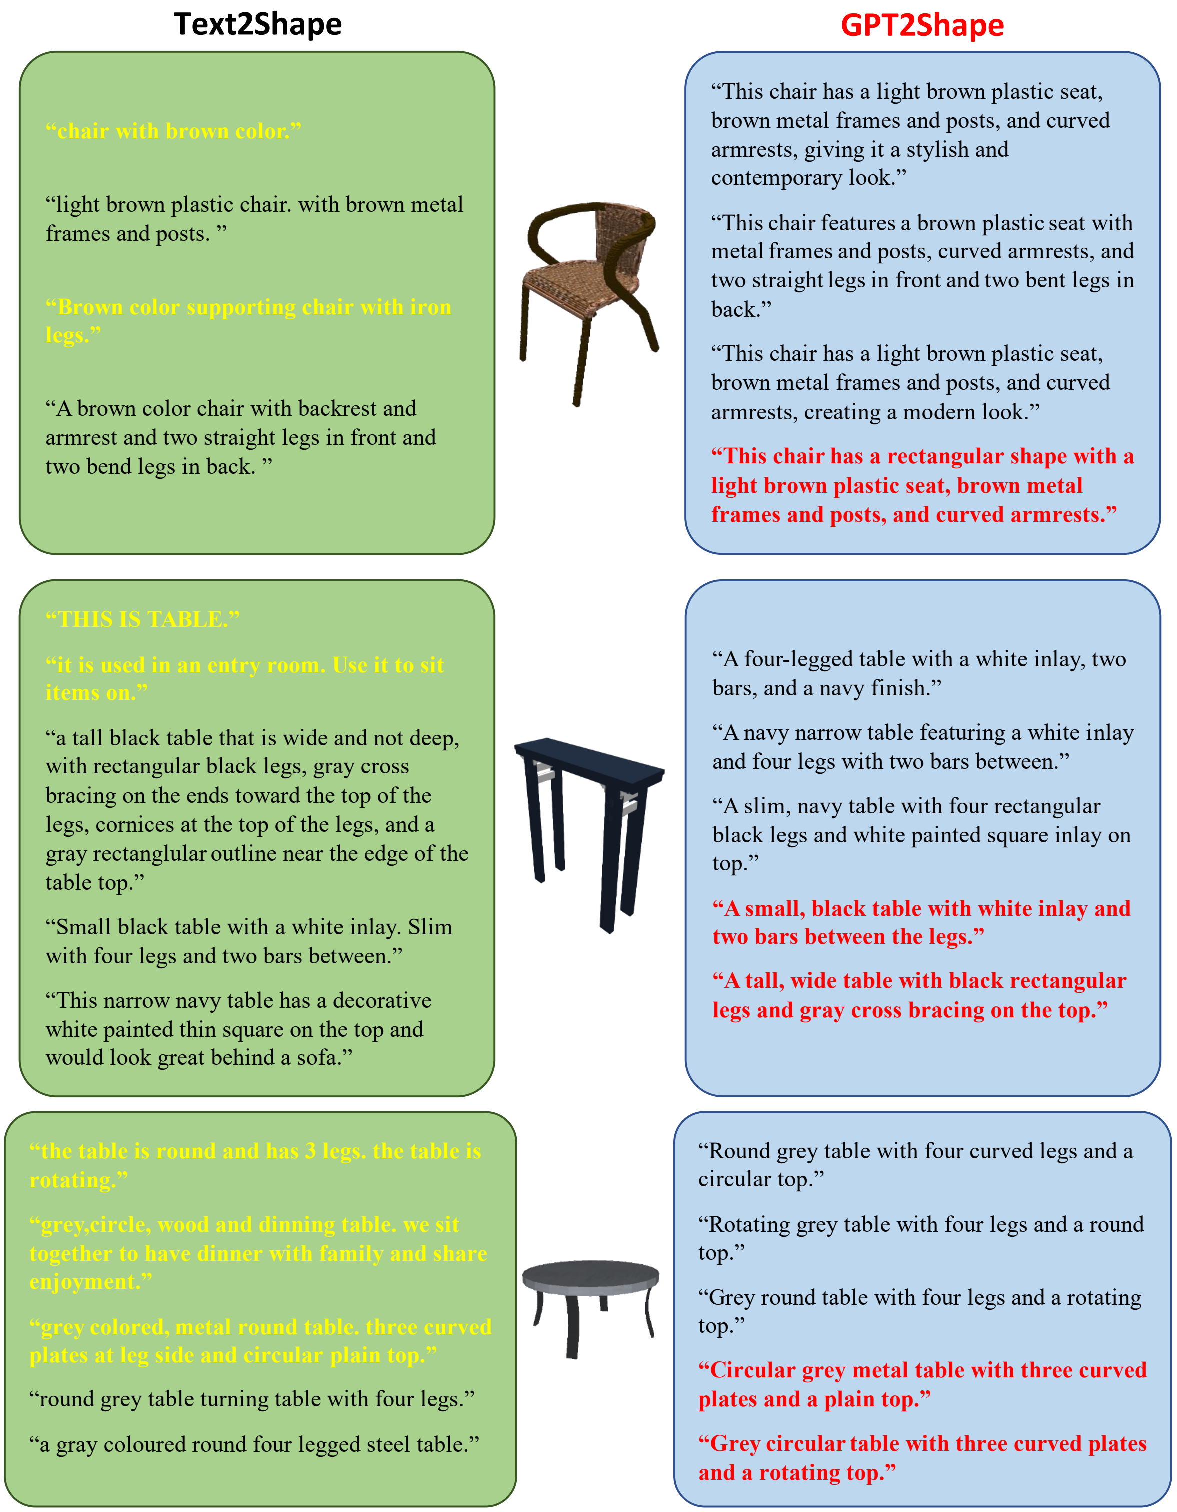


Figure 3. Three examples of wrong Text2Shape prompts which are improved but not completely corrected in GTP2Shape. The green box contains the original Text2Shape descriptions for the 3D shape in the middle. The blue box shows the rephrased text prompts of GPT2Shape. In yellow, we highlight the ambiguous or wrong descriptions of Text2Shape. In red, we highlight the wrong information in GPT2Shape descriptions.

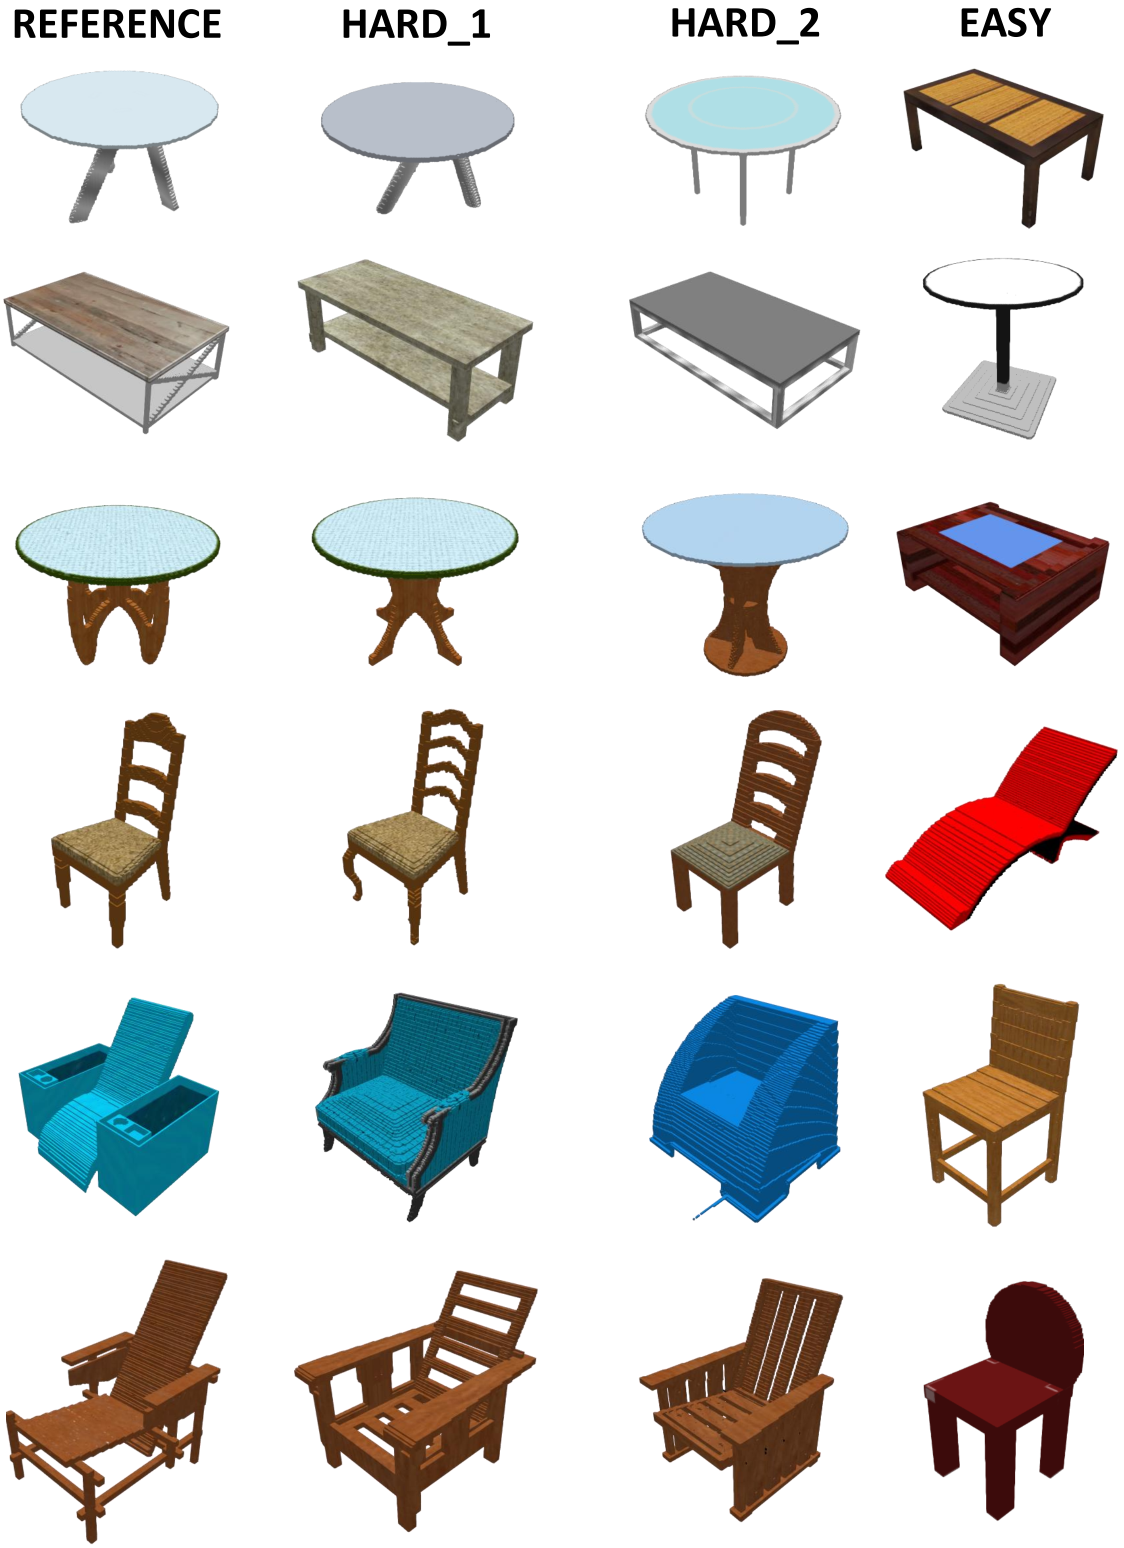


Figure 4. Collection of easy and hard distractors for some 3D shapes. Along each row, from left to right: the reference shape, the two closest shapes in the embedding space (*hard_1* and *hard_2*) and a randomly sampled shape from the *easy* distractors.

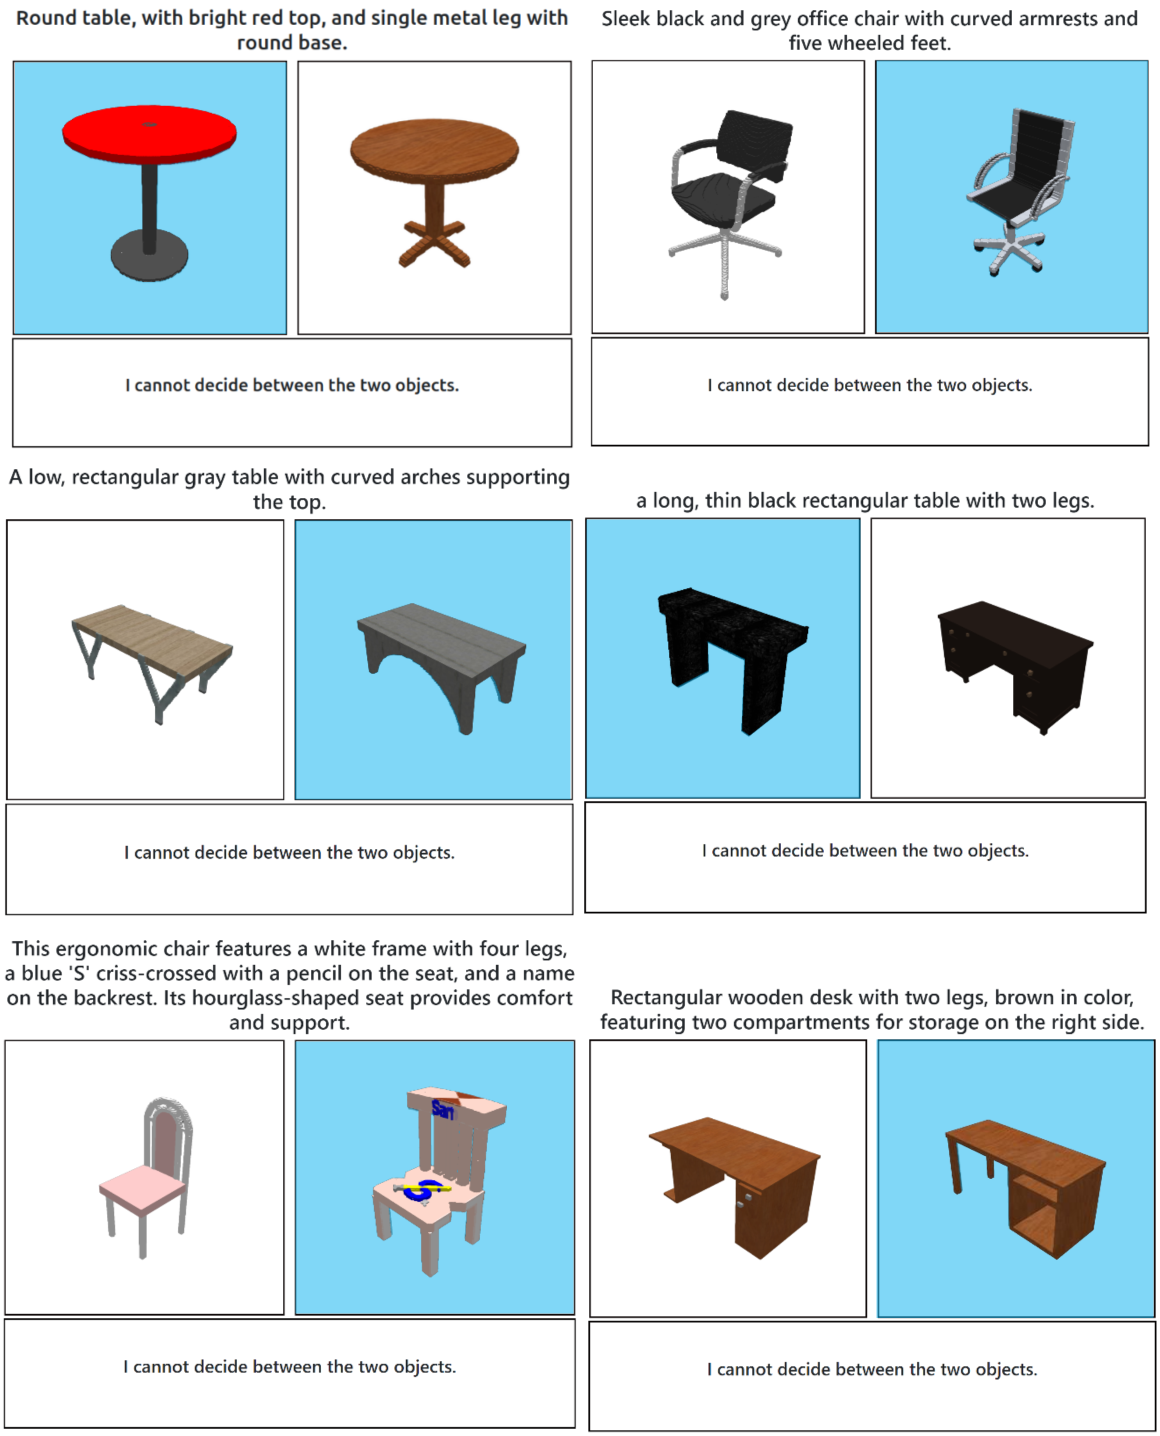


Figure 5. Example of triplets *shape-text-shape* which received unanimous approval from users. The unanimous response, for each triplet, is the 3D shape with the light blue background.

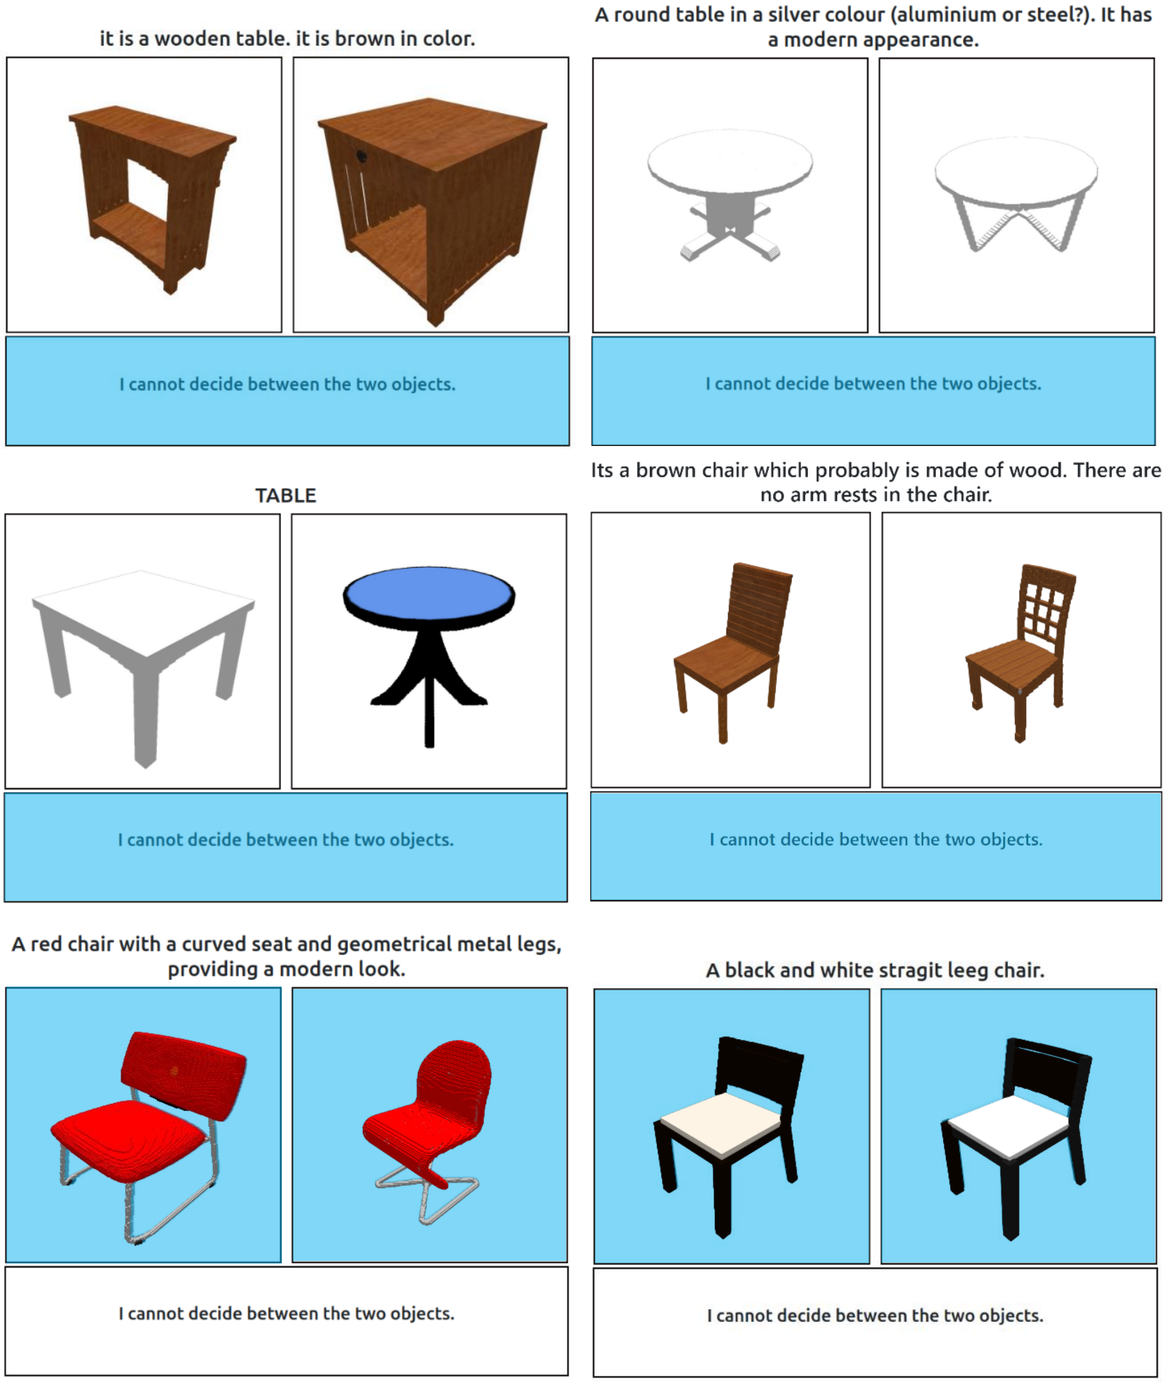


Figure 6. Example of triplets shape-text-shape which are unclear due to poor text prompts. In light blue, we highlight the responses given by at least one user.

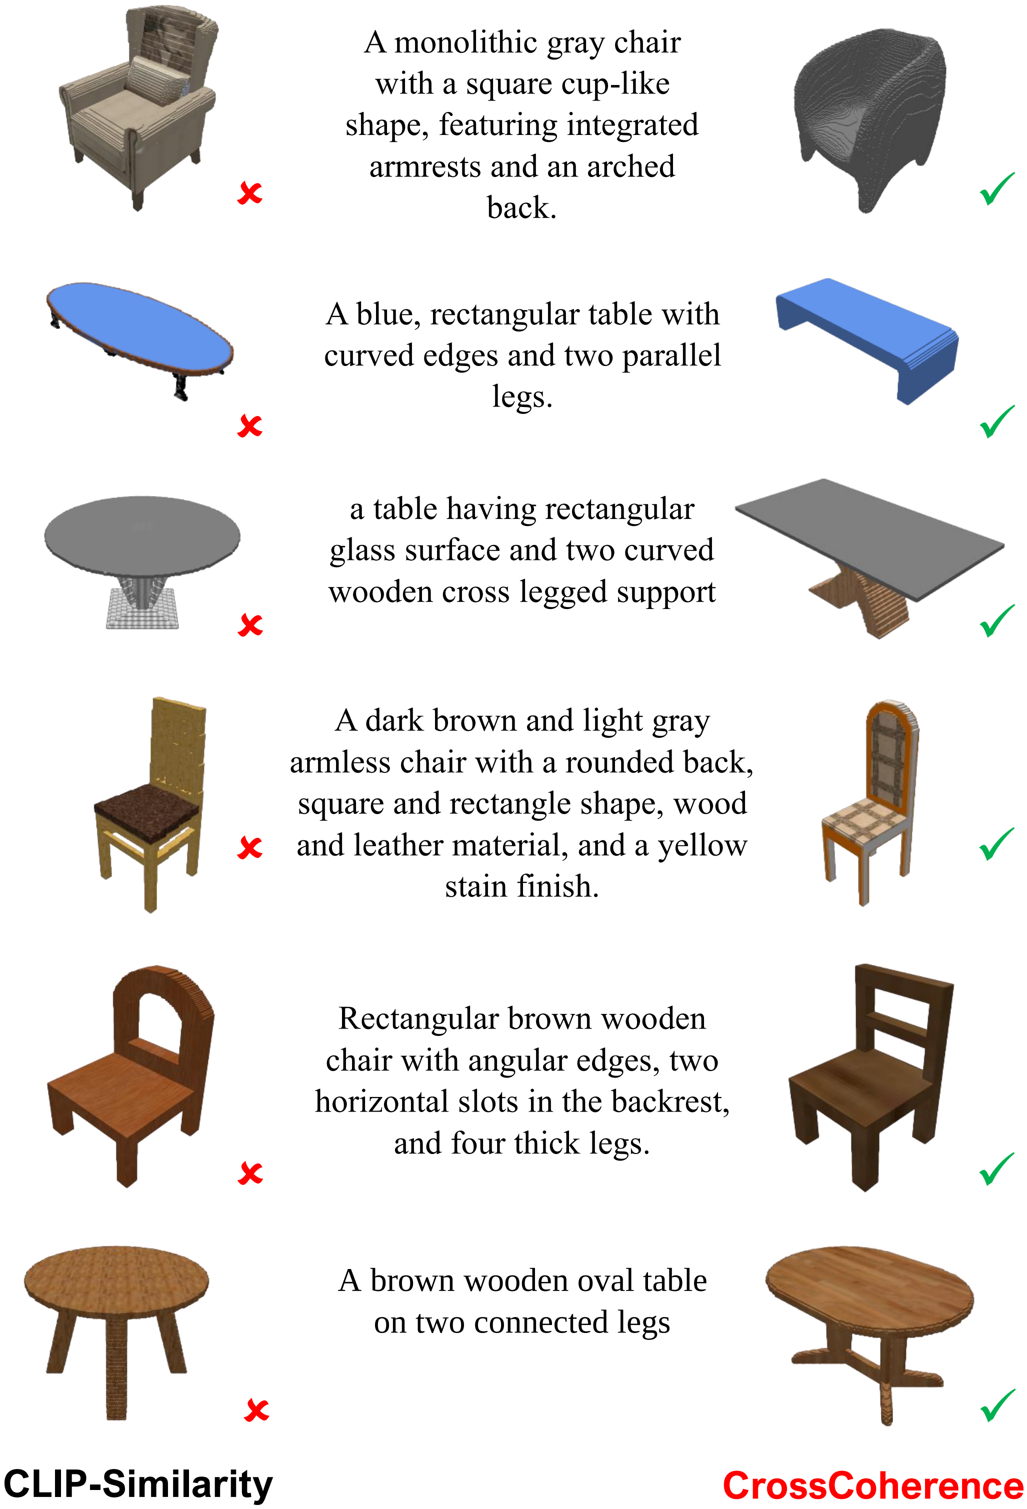


Figure 7. Qualitative results on the HST dataset, where the prediction from CrossCoherence is correct. The green check indicates the reference shape, associated with the prompt in the dataset, while the red cross identifies the distractor. For all these triplets, CrossCoherence selects the reference shape.

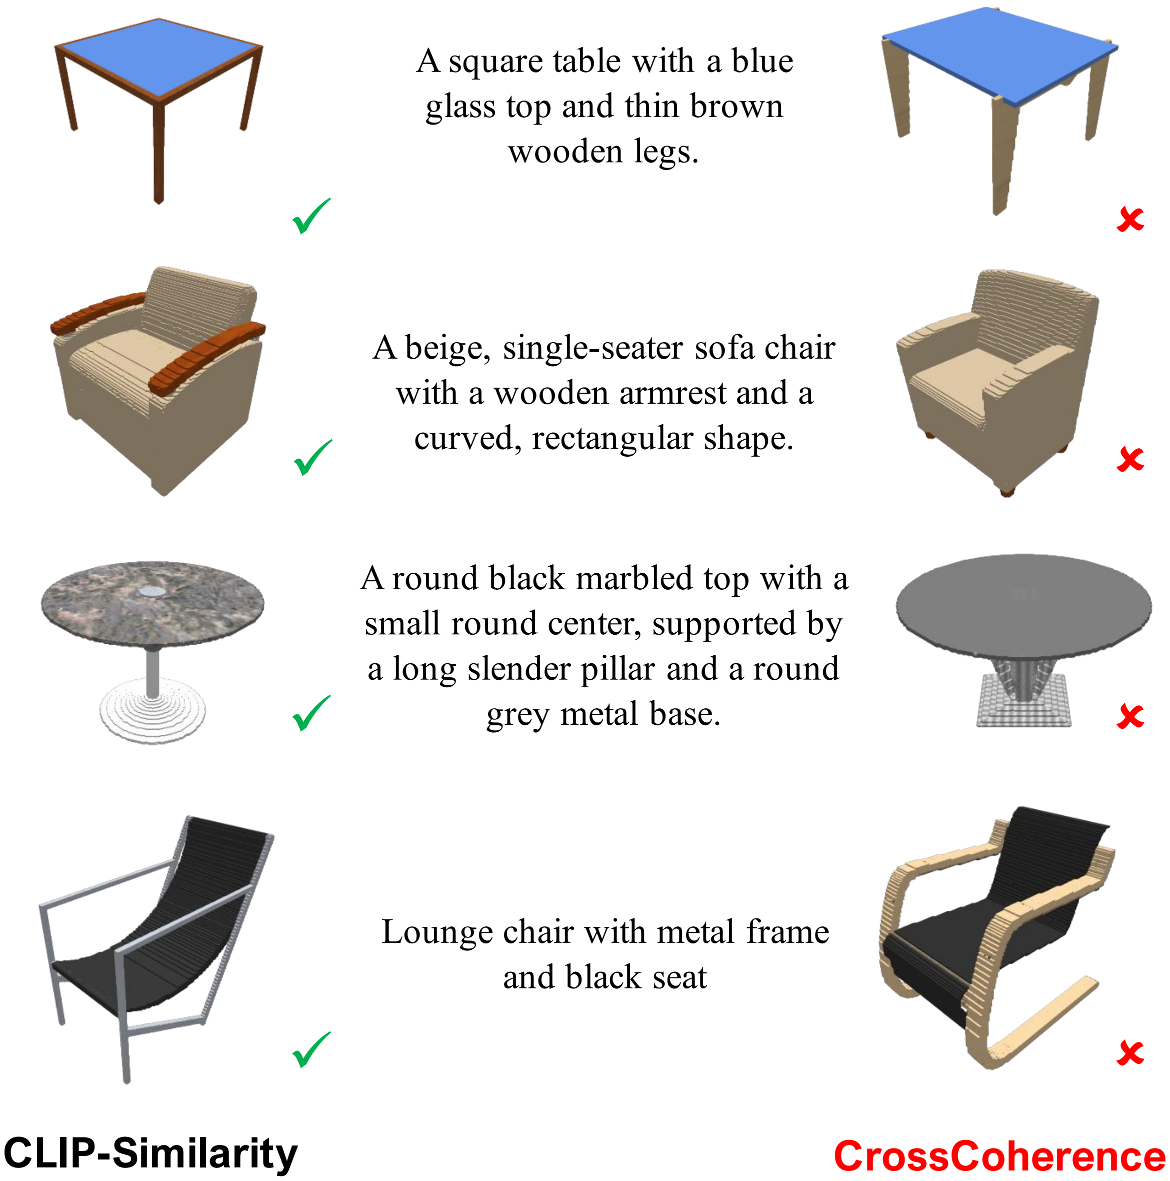


Figure 8. Qualitative results on the HST dataset, where the prediction from CrossCoherence is wrong. The green check indicates the reference shape, associated with the prompt in the dataset, while the red cross identifies the distractor. For all these triplets, CLIP-Similarity selects the reference shape.

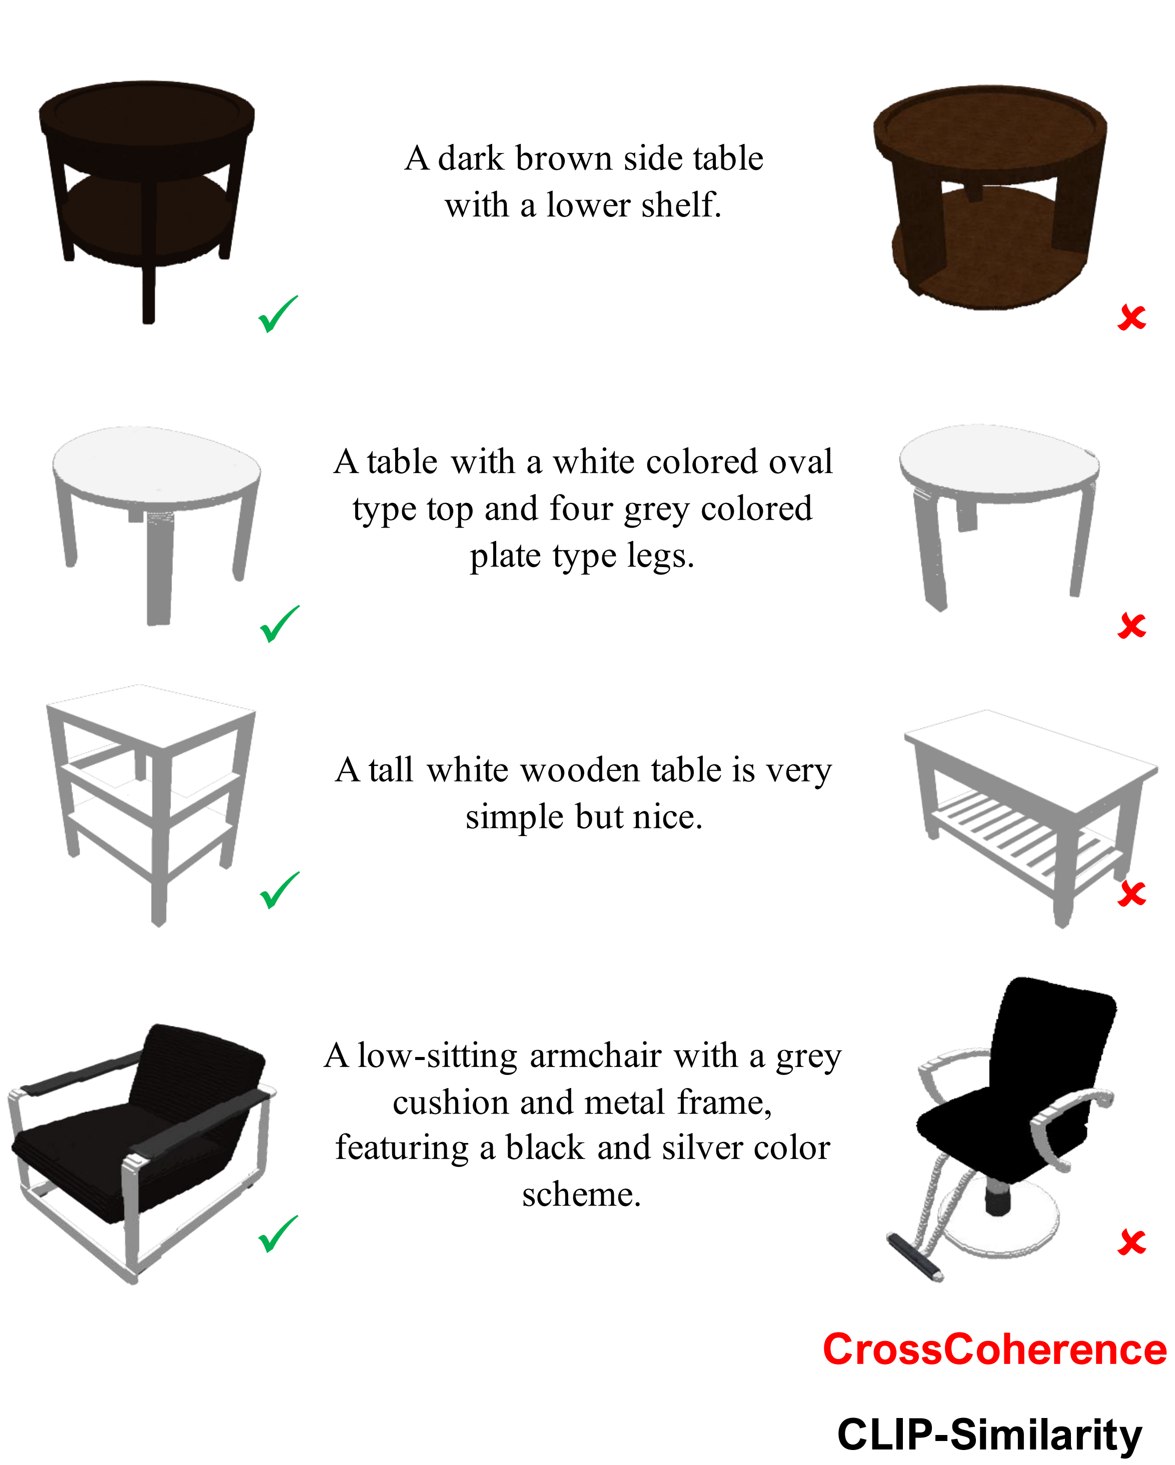


Figure 9. Qualitative results on the HST dataset, where both predictions from CLIP-Similarity and CrossCoherence are wrong. The green check indicates the reference shape, associated with the prompt in the dataset, while the red cross identifies the distractor. For all these triplets, CLIP-Similarity and CrossCoherence prefer the distractor shape.

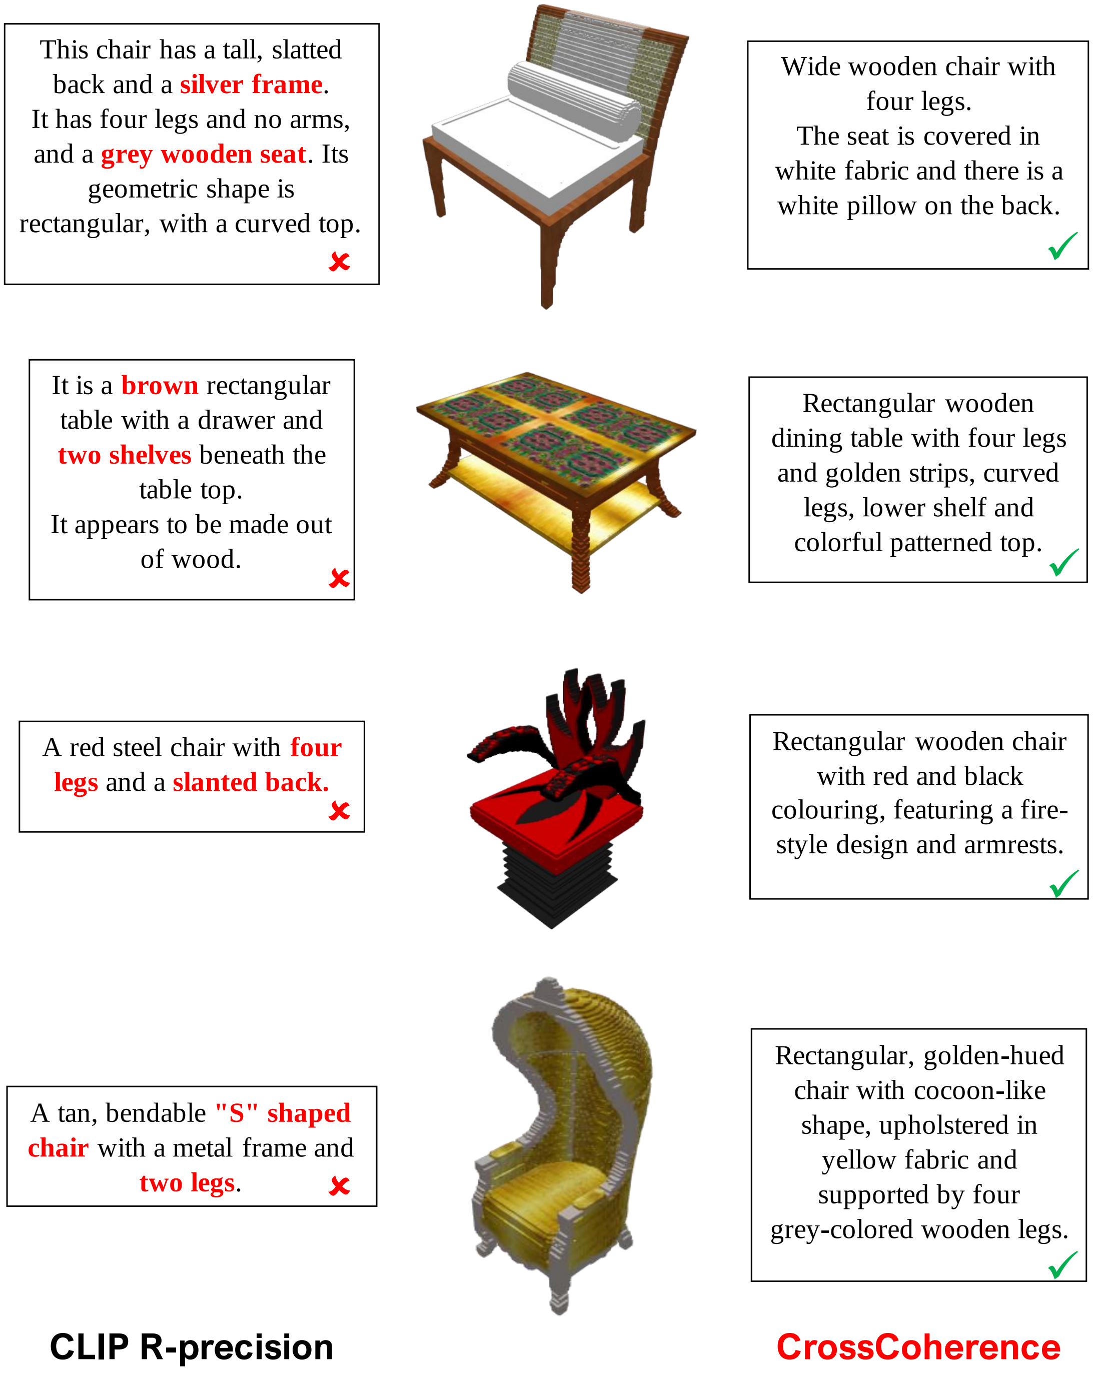


Figure 10. Qualitative results on the HST dataset, where the prediction from CrossCoherence is correct. The green check indicates the groundtruth text, associated with 3D shape in the middle, while the red cross identifies a wrong text prompt.

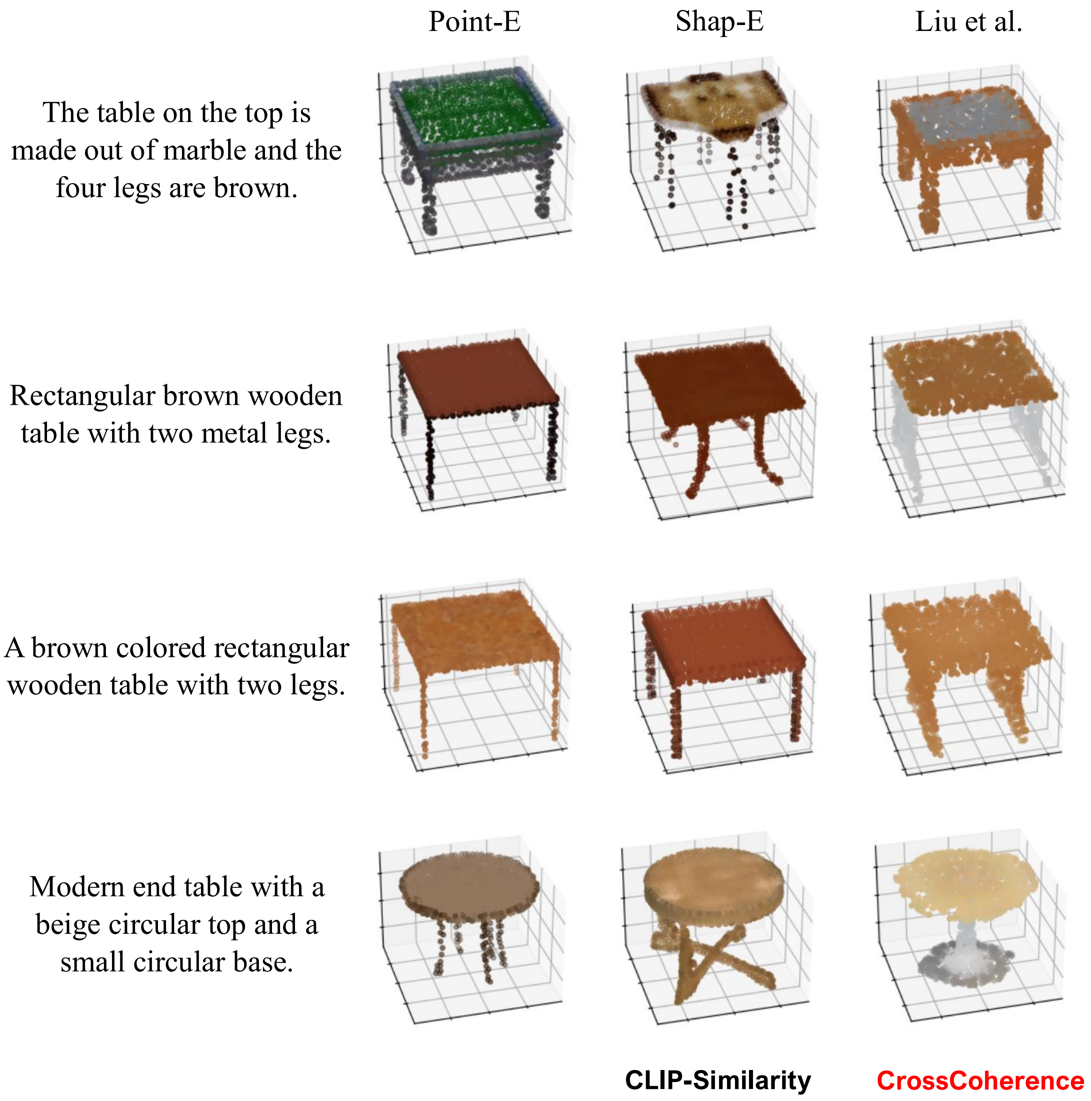


Figure 11. Examples of shapes generated by Point-E (left), Shap-E (center) and Liu et al. (right) for the given text prompt. As highlighted, for all these triplets, CLIP-Similarity prefers the shape in the middle while CrossCoherence the right one.

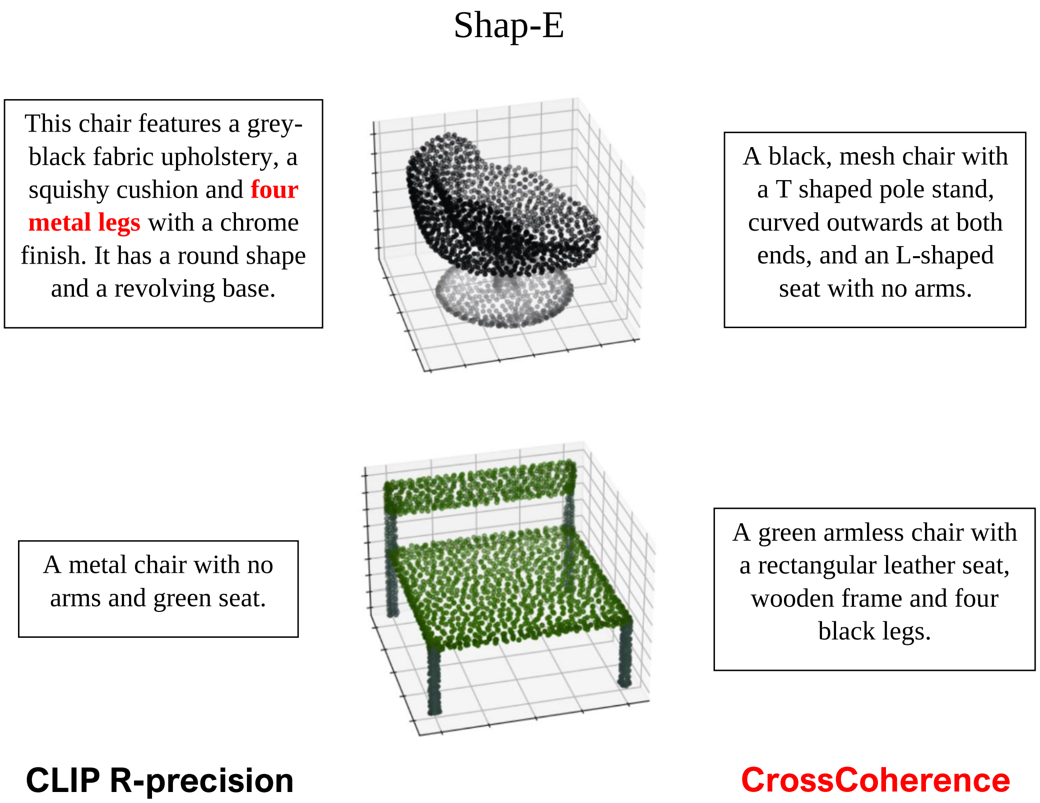


Figure 12. Examples of shapes generated by Shap-E with the corresponding text retrieved by CLIP R-precision, on the right, and CrossCoherence, on the left.
